# Supplementary material for: Learning to Predict Gradients for Semi-Supervised Continual Learning
Source: arXiv:2201.09196 source file (2024-01-31)
Supplement: Supplementary file 1 [file appendix.tex]

\section{Hyperparameters}
In this section, we report the hyperparameters for reproducing the experimental results.

This work follows the same experimental protocol used in \cite{Lopez_NIPS_2017,Luo_TPAMI_2019} to evaluate the proposed method on MNIST-R, MNIST-P, and iCIFAR-100, while it follows the same experimental protocol used in \cite{Ebrahimi_ECCV_2020} to evaluate the proposed method on CIFAR-100 and miniImageNet.
All hyperparameters that are used with the baselines are used with the proposed method as well.
In the following, we only focus on the hyperparameters that are related to the proposed method for clarity.

As introduced in \secref{sec:method} and \ref{sec:exp}, the hyperparameters include batch size of unlabeled images, threshold $p$, magnitude ratio $\alpha$, loss scale $\lambda$, architecture $h_{\omega}$, and batch size of unlabeled images.
Specifically, without loss of generality, we use MLP as the proposed gradient learner $h(\cdot;\omega)$ ($h_{\omega}$ for short) in this work. Assume the gradient is in $\mathbf{R}^{m}$, we denote (\textit{dimension of the 1st layer output}, \textit{dimension of the 2nd layer output}, \ldots, \textit{dimension of the penultimate layer output}) for simplicity. For instance, given $m=5$, architecture $(64, 16)$ indicates the MLP consists of three layers, the first one that is a linear operation with a coefficient matrix of size $5\times 64$, the second one that is with a coefficient matrix of $64\times 16$, and the last one that is with a coefficient matrix of size $16\times 5$.

\REVISION{Similar to other supervised learning techniques, few learning steps lead to poor predictive ability in gradient learning. To maintain the flexibility of the timing to update the model with predicted gradients, 
we start to apply the proposed method in the learning process after 50 learning steps in the GEM training scheme, and after 5 learning steps in the ACL training scheme.}

\REVISION{Note that restricted to the shared and private module design in ACL \cite{Ebrahimi_ECCV_2020}, which requires a fixed dimension of the input features, the batch size of unlabeled images has to be the same as the batch size of training samples, that is, 64.}

Here we provide the hyperparameters related to the proposed method, which are used to yield the experimental results in \tabref{tbl:conn_rota}, \ref{tbl:conn_perm}, \ref{tbl:conn_cifar}, \ref{tbl:acl_cifar100}, and \ref{tbl:acl_miniImageNet}, as reported in \tabref{tbl:hyper}. More details of the experiments can be found in the anonymous public repository \url{https://rb.gy/k8row9}.

\begin{table}[!t]
	\centering
	\caption{\label{tbl:hyper}
	    Hyperparameters w.r.t. the proposed method on various datasets. BS stands for the batch size of unlabeled images.
	}
% 	\vspace{-2ex}
	\adjustbox{width=1.0\columnwidth}{
% 	\begin{tabular}{L{18ex} C{9ex} C{9ex} C{9ex}}
	\begin{tabular}{l c c c c c c c}
		\toprule
		Dataset & Method & Backbone & BS & $p$ & $\alpha$ & $\lambda$ & $h_{\omega}$ \\ \midrule
		MNIST-R & GEM  & MLP & 4 & 0.15 & 0.001 & 0.30 & (64,16) \\
		MNIST-R & DCL  & MLP & 4 & 0.15 & 0.001 & 0.30 & (64,16) \\ \midrule
		MNIST-P & GEM & MLP & 4 & 0.15 & 0.001 & 0.50 & (64,16) \\
		MNIST-P & DCL & MLP & 4 & 0.15 & 0.001 & 0.49 & (64,16) \\ \midrule
		iCIFAR-100 & GEM & ResNet-18 & 4 & 0.30 & 0.005 & 2.00 & (128,32) \\
		iCIFAR-100 & DCL & ResNet-18 & 4 & 0.30 & 0.005 & 2.50 & (128,32) \\
		iCIFAR-100 & GEM & EffNet-B1 & 4 & 0.20 & 0.005 & 2.00 & (128,32) \\
		iCIFAR-100 & DCL & EffNet-B1 & 4 & 0.35 & 0.005 & 2.00 & (128,32) \\ \midrule
		CIFAR-100 & ACL  & AlexNet & 64 & 0.30 & 0.001 & 0.20 & (128,32) \\ \midrule
		miniImageNet & ACL & AlexNet & 64 & 0.35 & 0.001 & 0.15 & (128,32) \\
		\bottomrule
	\end{tabular}}
\end{table}
	
	\section{Training loss, validation accuracy, and fitness loss.} The losses and accuracy against tasks are shown in \figref{fig:loss_vs_accuracy}. We can see that the proposed method can improve the predictive ability with different models, \ie ResNet and EfficientNet. Moreover, the more predictive EfficientNet backbone can achieve higher accuracy with the proposed method. On the bottom row, the curves of the fitness loss vs. task show that the fitness loss (\ref{eqn:fit_loss}) across tasks is \REVISION{continuously minimized by the proposed gradient learner as the learning process moves on to various tasks.
	Also, the descent of fitness loss produced by EfficientNet is more significant than that of fitness loss produced by ResNet, which is consistent with the pattern in the loss curves and accuracies produced by EfficientNet and ResNet.}
	
	\input{depd/fig_loss_vs_accuracy}

% \vspace{1ex}
% \section{Ablation study}
% \REVISION{
% As introduced in the experimental set-up, the proposed method depends on five hyperparameters. This section shows the corresponding ablation studies and the results are shown in \fig~\ref{fig:abl}. As discussed in Section~\ref{sec:method}, $p$ reflects the trade-off between overwhelming and generalizing. As $p$ increases, the accuracy drops significantly. This is as expected in the earlier discussion. Moreover, we can observe that the architecture of the proposed gradient learner is more critical to the proposed method in terms of accuracy, BWT, and FWT, comparing to the other hyperparameters.}

% \input{depd/fig_ablation}

% \vspace{1ex}
\section{Cosine similarity}
\REVISION{
To find out how the proposed gradient learner correlates with the backbone network, we plot the cosine similarity between vanilla gradients and predicted gradients in \figref{fig:cosine}. Vanilla gradients are computed with the labels and inputs. They can be viewed as the ground truths for predicted gradients. It is ideal and desired that the gradient learner can predict pseudo gradients that are the same as underlying vanilla gradients (\ie the cosine similarities between vanilla gradients and predicted gradients are 1). The results shows that more discriminative features will lead to better gradient prediction in terms of the geometric relationship.}

\input{depd/fig_cosine}

\section{Confusion Matrix}
\REVISION{
To comprehensively understand the efficacy of the proposed predicted gradients, we visualize the confusion matrices of ResNet GEM and ResNet GEM with the proposed method on iCIFAR-100 as shown in \figref{fig:confusion}.
Observing and learning from extra unlabeled images mitigate overfitting. Thus, the performance on most tasks is improved.
}

\REVISION{
On the other hand, \tabref{tbl:noise} in the paper shows that using random noise as predicted gradients yields higher BWT than the other settings. This is because the random noise disturbs the learning process of early tasks, which leads to low accuracies as shown in \figref{fig:confusion_u} and \ref{fig:confusion_n}. According to the definition of BWT \cite{Lopez_NIPS_2017}, \ie $\frac{1}{T-1}\sum_{i=1}^{T-1} R_{T,i}-R_{i,i}$, $R_{i,i}$ is far lower than $R_{T,i}$ so that the corresponding BWT is a large number.
}

\input{depd/fig_anal_confusion_base_proposed}

\begin{figure*}[!t]
	\centering
	\begin{minipage}[t]{0.40\textwidth}
        \centering
        \vspace{0pt}
        \includegraphics[width=1\linewidth]{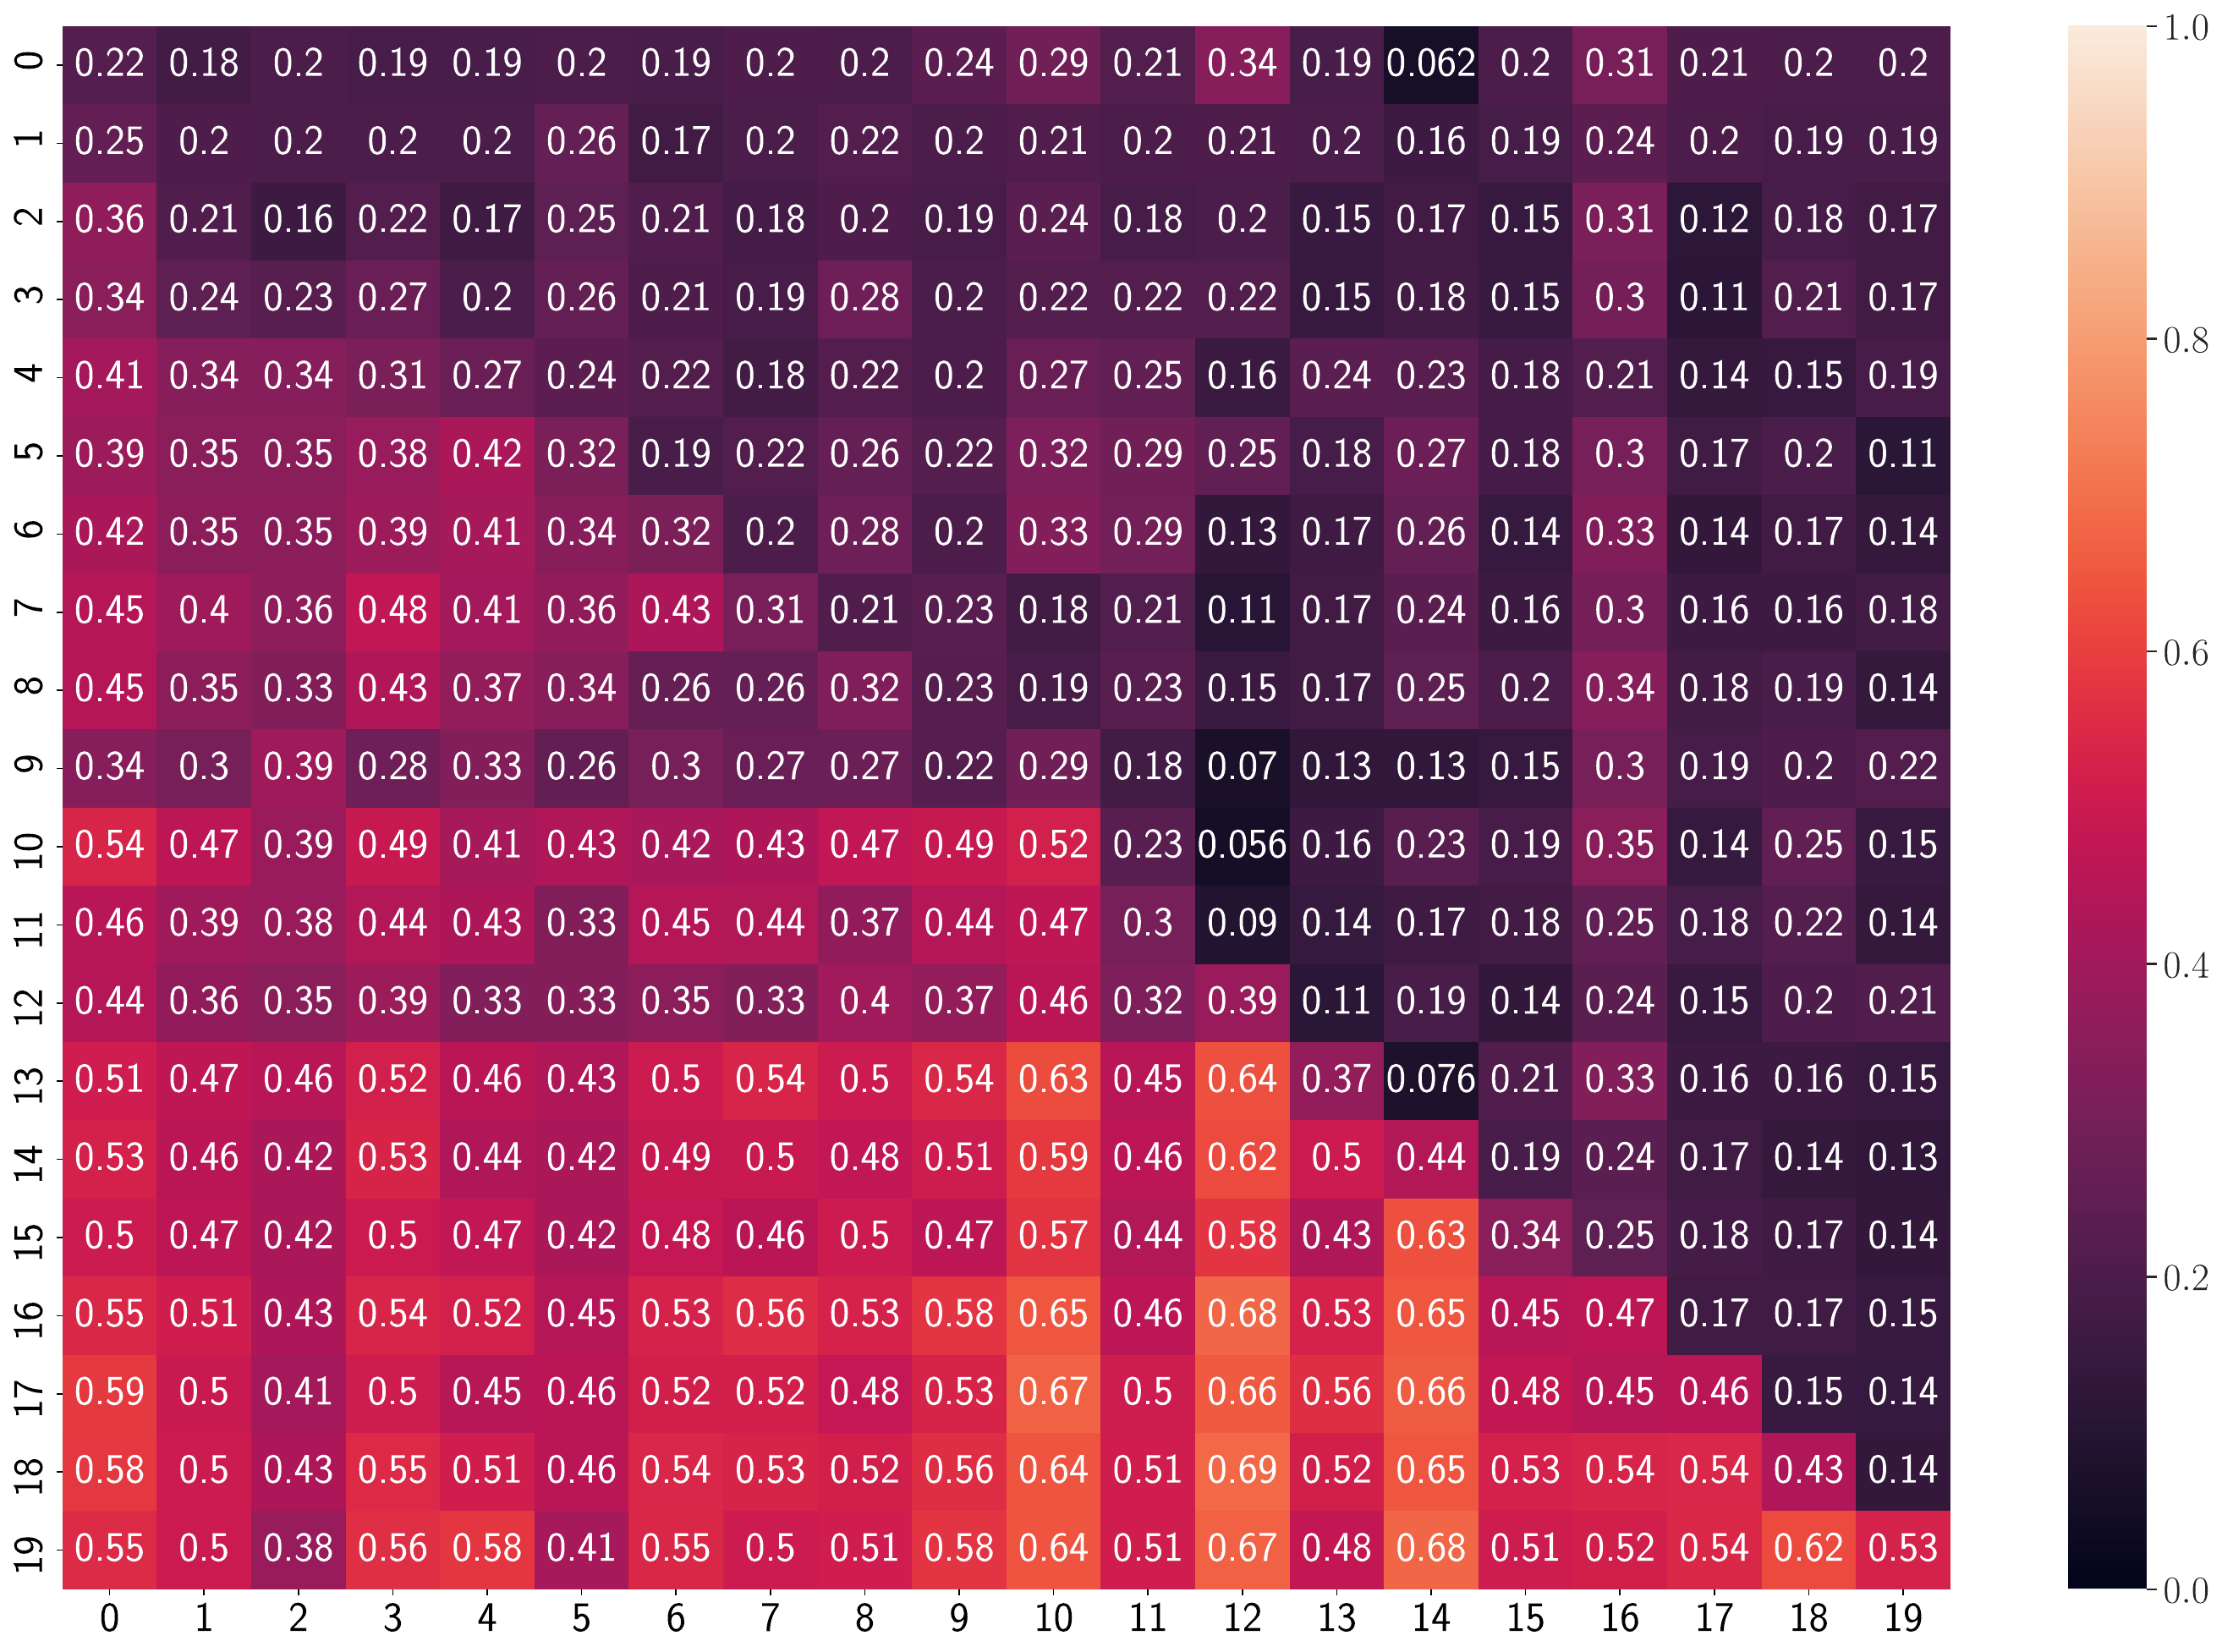}
        \caption*{ResNet GEM $\mathcal{U}(-1,1)$}
    \end{minipage} \hfill
    \begin{minipage}[t]{0.40\textwidth}
        \centering
        \vspace{0pt}
        \includegraphics[width=1\linewidth]{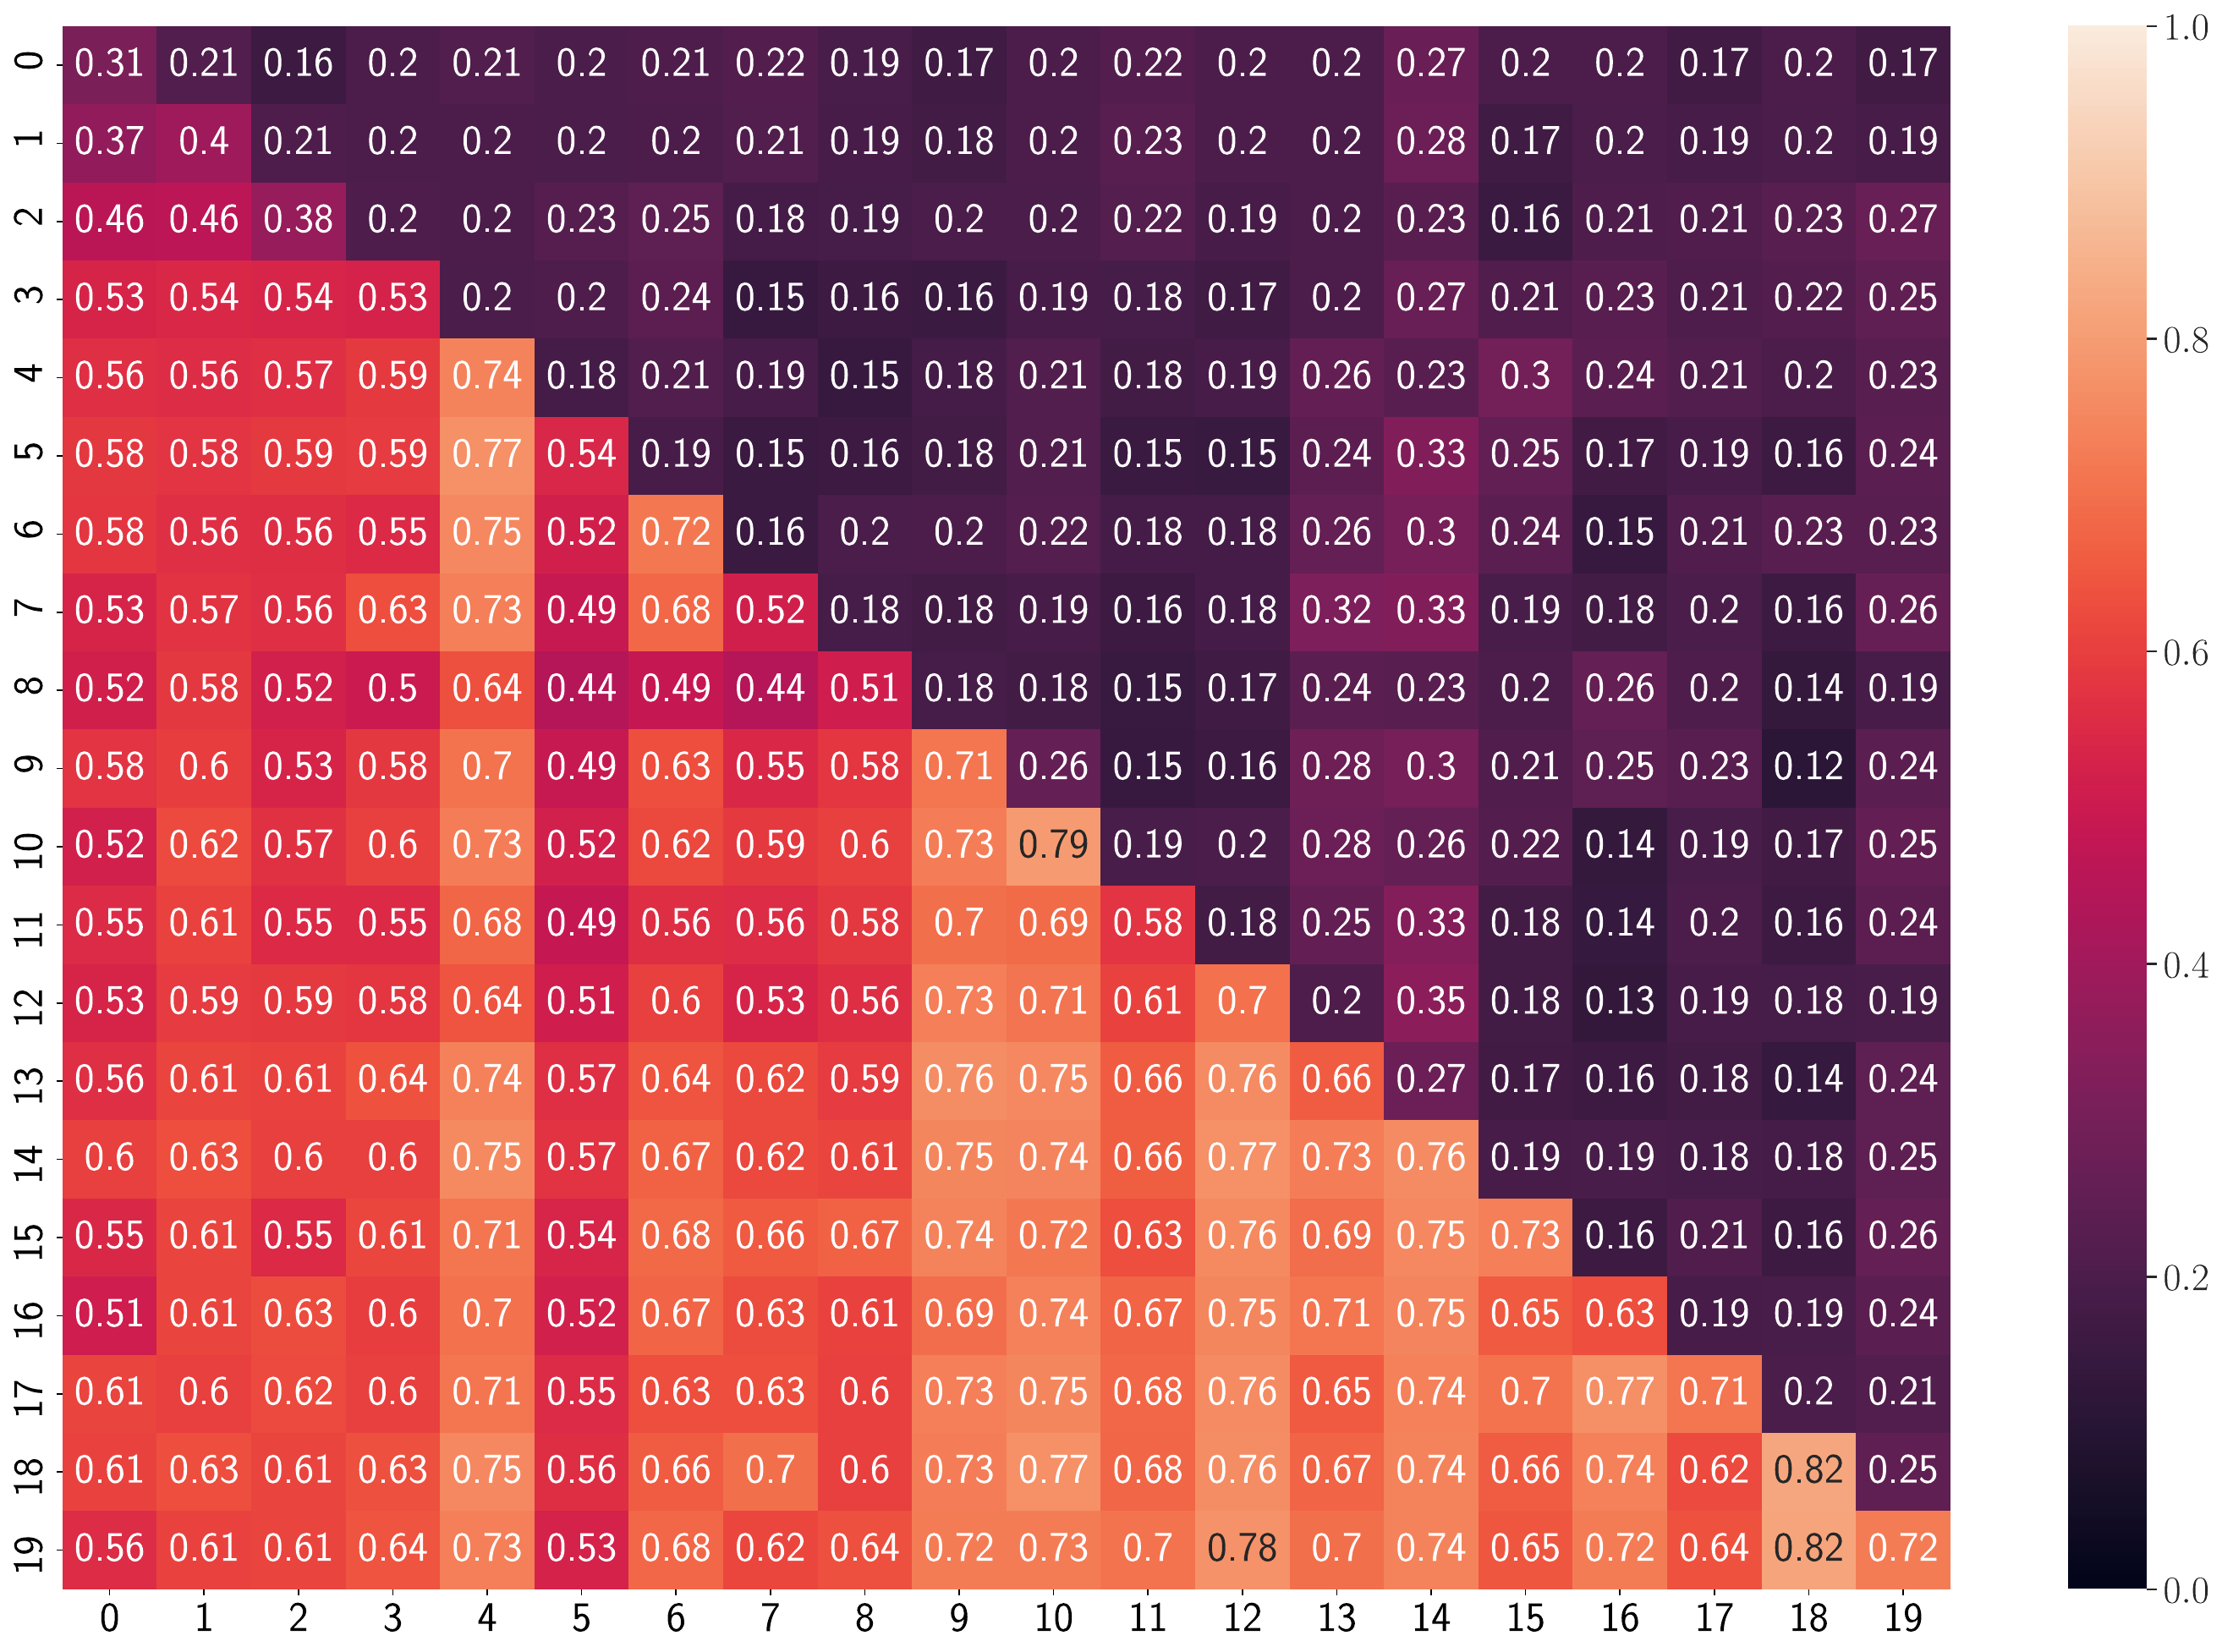}
        \caption*{ResNet GEM $\mathcal{U}(-1,1)$ + proposed}
    \end{minipage}
	\caption{\label{fig:confusion_u}
    	Confusion matrix using random noise as predicted gradients. The noise follows a uniform distribution $\mathcal{U}(-1,1)$.
    % 	that is evaluated at every training stage for all the tasks by substituting the noise for the predicted gradients.
	}
\end{figure*}

\input{depd/fig_anal_confusion_noise_n}
